# Supplementary material for: Private Online Prediction from Experts: Separations and Faster Rates
Source: arXiv:2210.13537 source file (2023-06-29)
Supplement: Supplementary file 1 [file realizable-appendix-experts.tex]

\section{Additional details for~\Cref{sec:upper-bounds-realizable}}

\subsection{A binary-tree based algorithm}
\label{sec:bt-experts}
In this section, we present another algorithm which achieves the optimal regret for settings with zero-expert loss. Instead of using sparse-vector, this algorithm builds on the binary tree mechanism. The idea is to repetitively select $O(\mathsf{poly}(\log(dT)))$ random good experts and apply the binary tree to calculate a private version of their aggregate losses. Whenever all of the chosen experts are detected to have non-zero loss, we choose a new set of good experts. Similarly to~\cref{alg:SVT-zero-loss}, each new phase reduces the number of good experts by a constant factor as an oblivious adversary does not know the choices of the algorithm, hence there are only $O(\mathsf{poly}(\log(dT)))$ phases.

We provide a somewhat informal description of the algorithm in~\cref{alg:Bin-tree-zero-loss}. This algorithm also achieves regret $O(\mathsf{poly}(\log(dT))/\diffp)$ in the realizable case. We do not provide a proof as it is somewhat similar to that of~\cref{thm:ub-realizable}.
\begin{algorithm}
	\caption{Binary-tree algorithm for zero loss experts (sketch)}
	\label{alg:Bin-tree-zero-loss}
	\begin{algorithmic}[1]
		%\REQUIRE Data points $\Ds=(\ds_1, \ldots, \ds_n)\in \domain^n$,
		%constraint set $\xdomain$,
		%step size $\ss$, initial point $x_0$;
		\STATE Set $k=0$ and $B=  O(\mathsf{poly}(\log(dT)))$
        \WHILE{$t \le T$\,}
            \STATE Use the exponential mechanism with score function $s(x) = \sum_{i=1}^t \ell_i(x)$ to privately select a set $S_k$ of $B$ experts from $[d] \setminus \cup_{0 \le i \le k} S_i$
            \STATE Apply binary tree for each expert $x \in S_k$ to get private aggregate estimates for $ \sum_{i=1}^t \ell_i(x)$ for every $t \in [T]$
            \STATE Let $\hat c_{t,x}$ denote the output of the binary tree for expert $x \in S_k$ at time $t$ 
            \WHILE{there exists $x \in S_k$ such that $\hat c_{t,x} \le O(\mathsf{poly}(\log(dT))/\diffp)$}
                \STATE Receive $\ell_t : [d] \to [0,1]$
                \STATE Choose $x_t \in S_k$ that minimizes $\hat c_{t,x}$
        	    \STATE Pay error $\ell_t(x_t)$
        	    \STATE $t = t+1$
            \ENDWHILE
            \STATE $k = k + 1$
        \ENDWHILE
	\end{algorithmic}
\end{algorithm}

\subsection{Proof for~\Cref{thm:ub-realizable-ada}}
\label{sec:proof-ub-realizable-ada}
First we prove privacy. Note that $\bar L\opt$ can change at most $\log(T)$ times as $L\opt \le T$. Therefore, we have at most $\log(T)$ applications of~\Cref{alg:SVT-zero-loss}. Each one of these is $\diffp/(2\log(T))$-DP. Moreover, since we have at most $K$ applications of the exponential mechanism in~\Cref{alg:SVT-zero-loss}, we have at most $K \log(T)$ applications of the Laplace mechanism in~\Cref{alg:SVT-ada}. Each of these is $\diffp/2K\log(T)$-DP. Overall, privacy composition implies that the final privacy is $\diffp$-DP.

Now we prove utility. \Cref{alg:SVT-ada} consists of at most $\log(T)$ applications of~\Cref{alg:SVT-zero-loss} with different values of $\bar L\opt$. We will show that each of these applications incurrs low regret.
    Consider an application of~\Cref{alg:SVT-zero-loss} with $\bar L\opt$. If $\bar L\opt \ge L\opt$, then~\Cref{thm:ub-realizable} implies that the regret is at most $$O\left( \bar L\opt \log(d/\beta_0) + \frac{\log^2(d) + \log(T/\beta_0) \log(d/\beta_0)}{\diffp_0}  \right).$$ 
    Now consider the case where $\bar L\opt \le L\opt$. We will show that~\Cref{alg:SVT-ada} will double $\bar L\opt$ and that the regret of~\Cref{alg:SVT-zero-loss} up to that time-step is not too large.
    Let $t_0$ be the largest $t$ such that $\min_{x \in [d]} \sum_{t=1}^{t_0} \ell_t(x) \le \bar L\opt$. Note that up to time $t_0$, the best expert had loss at most $\bar L\opt$ hence the regret up to time $t_0$ is $$O\left( \bar L\opt \log(d/\beta_0) + \frac{\log^2(d) + \log(T/\beta_0) \log(d/\beta_0)}{\diffp_0}  \right).$$ 
    Now let $t_1$ denote the next time-step when~\Cref{alg:SVT-zero-loss} applies the exponential mechanism. Sparse-vector guarantees that in the range $[t_0,t_1]$ the algorithm suffers regret at most $O\left( \bar L\opt  + \frac{\log(d) + \log(T/\beta_0) }{\diffp_0}  \right)$. Moreover, the guarantees of the Laplace mechanism imply that at this time-step, $\bar L_t \ge \bar  L\opt - 5K\log(1/\beta_0)/\diffp_0$ with probability $1-\beta_0$, hence~\Cref{alg:SVT-ada} will double $\bar L\opt$ and run a new application of~\Cref{alg:SVT-zero-loss}. Overall, an application of~\Cref{alg:SVT-zero-loss} with $\bar L\opt \le L\opt$ results in regret $(L\opt + \frac{1}{\diffp_0}) \cdot \mathsf{poly} (\log \frac{Td}{\beta_0})$ and doubles $\bar L\opt$. Finally, note that if $\bar L\opt \ge L\opt + 5\log(1/\beta_0)/\diffp_0$ then with probability $1-\beta_0$ the algorithm will not double the value of $\bar L\opt$. As each application of ~\Cref{alg:SVT-zero-loss} has regret $$O\left( \bar L\opt \log(d/\beta_0) + \frac{\log^2(d) + \log(T/\beta_0) \log(d/\beta_0)}{\diffp_0}  \right),$$ and $\bar L\opt$ is bounded by $L\opt + 5\log(T/\beta_0)/\diffp_0$ with probability $1 - O(\beta_0)$. Overall, the failure probability is $O(T \beta_0) = O(\beta)$. \ha{go over this proof again..}
