# Supplementary material for: Private Online Prediction from Experts: Separations and Faster Rates
Source: arXiv:2210.13537 source file (2023-06-29)
Supplement: Supplementary file 3 [file realizable-appendix-OCO.tex]

\section{Missing proofs for~\Cref{sec:dp-oco}}

\subsection{Proof of~\Cref{thm:DP-OCO}}
\label{sec:proof-dp-oco}
Let $x_1,\dots,x_T$ be the experts chosen by the algorithm.
    First, \Cref{thm:ub-realizable-ada} implies that this algorithm obtains the following regret with respect to the best expert
    \begin{equation*}
        \sum_{t=1}^T \ell_t(x_t) - L^{\opt}_{\mathsf{experts}} \le (L^{\opt}_{\mathsf{experts}}  + \frac{1}{\diffp})  \cdot O\left( \mathsf{poly} (d\log \frac{DT}{\rho\beta}) \right),
    \end{equation*}
    where $L^{\opt}_{\mathsf{experts}} = \min_{x \in \mc{X}^\rho_{\mathsf{experts}}} \sum_{t=1}^T \ell_t(x)$. Since $\ell_t$ is $L$-Lipschitz for each $t \in [T]$, we obtain that 
    \begin{equation*}
    | L\opt - L^{\opt}_{\mathsf{experts}} |
        = |\min_{x \in \mc{X}} \sum_{t=1}^T \ell_t(x) - \min_{x \in \mc{X}^\rho_{\mathsf{experts}}} \sum_{t=1}^T \ell_t(x) |  
        \le T L  \rho.
    \end{equation*}
    Overall this gives
     \begin{equation*}
        \sum_{t=1}^T \ell_t(x_t) - L^{\opt} 
        \le (L^{\opt} + TL\rho + \frac{1}{\diffp}) \cdot O\left( \mathsf{poly} (d\log \frac{DT}{\rho\beta}) \right).
    \end{equation*}
    Setting $\rho = 1/(LT)$ proves the claim.
